# Supplementary material for: Pre-train or Annotate? Domain Adaptation with a Constrained Budget
Source: arXiv:2109.04711 source file (2022-05-13)
Supplement: Supplementary file 1 [file appendix.tex]

% To facilitate our comparison across different setups, we need to prepare multiple datasets for different purposes. In this section, we will present the details of data preparation, which consists of two parts, in-domain data annotation for supervised methods and unlabelled procedural corpus collection for unsupervised methods. 

% \subsection{In-Domain Data Annotation}
% There are two reasons to annotate two new datasets: 1) experiment with the supervised setup; 2) facilitate the research on procedural text on two related-but-new domains. We will describe the annotation detail here and make a table to show data stats.

\section{Procedural Corpus Collection}
\label{sec:app_corpus}
\paragraph{PubMed Articles}
The first source is PubMed articles, and we chose to work with PubMed data because it is a large repository of articles containing descriptions of experimental procedures that can be freely accessed and shared. Specifically, we extracted paragraphs describing procedures (including chemical synthesis procedures) from the {\em Materials and Methods} section of articles within the open access subset of PubMed.  XML files containing full-text of the articles were downloaded from NCBI\footnote{\url{https://www.ncbi.nlm.nih.gov/}}, and they were processed to extract the PubMed ID for each article in addition to all paragraphs within a section of a paper with the title ``Materials and Methods.'' 

To filter out paragraphs within the materials and methods section that are not describing procedures, we developed a scientific discourse tagger using the dataset SciSeg \citep{Dasigi2017ExperimentSI}.  This dataset annotates clauses within PubMed articles with a set of discourse labels: {\tt \{Goal, Fact, Result, Hypothesis, Method, Problem, Implication\}}. We fine-tuned SciBERT \citep{Beltagy2019SciBERTAP} using this dataset to automatically label PubMed sentences, achieving an average F1 score of 72.65\% in a  five-fold cross validation.

After training, we ran the scientific discourse tagger described above on each paragraph extracted from a {\em Materials and Methods}.  We consider a paragraph to describe a valid procedure if at least 40\% of clauses are labeled as {\tt Method}.  The threshold was obtained by manual inspection of the randomly sampled subset of the data.

In total the PubMed OpenAccess subset contains 2,542,736 articles, of which about 650k contain a {\em Materials and Methods} section.  After filtering as described above, we retained a set of 1,785,923 paragraphs describing procedures.  Based on a manual inspection of the extracted paragraphs, we estimate that 92\% consist of instructions for carrying out experimental procedures.

\paragraph{Chemical Patents}
The second source of procedural text is the patent data as chemical patents include the detailed procedures of chemical synthesis. Similarly, to extract paragraphs describing experimental steps from the {\em Description} section of chemical patents, we first downloaded US patent data (1976-2016) from USPTO\footnote{\url{https://www.uspto.gov/learning-and-resources/bulk-data-products}} and European data (1978-2020) from EPO\footnote{\url{https://www.epo.org/searching-for-patents/data/bulk-data-sets.html}} as XML files. Then we applied the reaction extractor developed by \citet{Lowe2012ExtractionOC}, which is a trained Naive Bayes classifier, to all our patent corpus. Note that the US patent data has two subsets, "Grant" (1976-2016) and "Application" (2001-2016). The "Application" subset contains the "Grant" subset for the same year, so we only use the US patents from the "Application" subset for those overlapping periods (2001-2016). As a result, we can get 2,435,999 paragraphs from US patents and 4,039,605 paragraphs from European patents. What's more, as our focus is the English data, we used the tool \textbf{langid}\footnote{\url{https://github.com/saffsd/langid.py}} to identify the source language for each extracted paragraph, and only kept English data, which has 3,671,482 paragraphs (90.9\%).

% \paragraph{Recipes}
% The third source we selected is the recipe data, which is a standard procedural text as every cooking step is listed separately. For this source, we directly used the text component of Recipe1M+ dataset \citep{Marn2019Recipe1MAD} as it is the largest recipe dataset publicly available. The recipes in this dataset were scraped from famous cooking websites and pre-processed with a pipeline to get the clean text. The number of recipes in this dataset is 1,029,720.

\section{Data Annoataion}
\label{sec:data_anno}
To facilitate the comparison between the pre-training based approach and the supervised domain adap-tation approach, we created two new datasets \textsc{PubMedM\&M} and \textsc{ChemSyn} in the domain of scientific articles and chemical patents mainly following the annotation scheme of the Wet Lab Protocols (WLP) framework \citep{Kulkarni2018AnAC}. In WLP, there are 18 Entity types (including the Action) and 14 Relation types. On top of it, we supplemented four new Entity types (\textsc{Company}, \textsc{Software}, \textsc{Collection(Data)} and \textsc{Info-Type}) and one new Relation type (\textsc{Belong-To}) due to two key features of our corpus: 1) Scientific articles usually specify the provenance of reagents for better reproducibility; 2) Other than wet-lab experiments, our corpus also includes the detail of data processing/analysis and computer-simulated experiments. 
For the \textsc{PubMedM\&M} dataset, we annotated a corpus of 191 of the procedural text paragraphs extracted from a subset of PubMed articles. Similarly, for the \textsc{ChemSyn} dataset, we annotated 600 sampled chemical synthesis-related paragraphs obtained from chemical patents. The statistics of these two datasets are presented in Table \ref{tab:mm_stats} and Table \ref{tab:chemsyn_stats} respectively.

The annotation process is conducted with BRAT annotation tool, and it consists of two steps. In the first step, each file is distributed to two annotators, and they will annotate the file independently. Then in the second step, the coordinator will discuss the annotation with each annotator making sure their annotation follows the guideline and dissolve the disagreement. We double-annotated all files in the \textsc{PubMedM\&M} dataset and half of the files in the \textsc{ChemSyn} dataset. As for the inter-annotator agreement (IAA) score, we treat the annotation from one of the two annotator as the gold label, and the other annotation as the predicted label, and then use the F1 scores of Entity(Action) and Relation evaluations as the final inter-annotator agreement scores, which can be found in Table \ref{tab:iaa_results}. We can see that the \textsc{ChemSyn} dataset has higher IAA scores for two potential reasons: 1) we annotated the \textsc{PubMedM\&M} dataset first, so the annotators might be more experienced when they annotated the \textsc{ChemSyn} dataset; 2) the \textsc{PubMedM\&M} dataset contains more diverse content like wet lab experiments or computer simulation procedures while the \textsc{ChemSyn} dataset is mainly about chemical synthesis.

\begin{table}[h!]
\small
\begin{center}
% \setlength\tabcolsep{3pt}
\begin{tabular}{lccc}
\thickhline  & Total & per Protocol & per Sentence \\ \hline
\# of sentences & 1508 & 7.90 & - \\ 
\# of words &  29121 & 152.47 & 19.31 \\ \hline
\# of entities &  9845 & 51.54 & 6.53 \\ 
\# of relations &  8987 & 47.05 & 5.96 \\ 
\# of actions  &  2286 & 11.97 & 1.52  \\ 
\thickhline
\end{tabular}
\end{center}
\caption{\label{tab:mm_stats}  Statistics of the \textsc{PubMedM\&M} Corpus.}
\end{table}

\begin{table}[h!]
\small
\begin{center}
% \setlength\tabcolsep{3pt}
\begin{tabular}{lccc}
\thickhline  & Total & per Protocol & per Sentence \\ \hline
\# of sentences &  \\ 
\# of words &   \\ \hline
\# of entities &   \\ 
\# of relations &   \\ 
\# of actions  &    \\ 
\thickhline
\end{tabular}
\end{center}
\caption{\label{tab:chemsyn_stats}  Statistics of the \textsc{ChemSyn} Corpus.}
\end{table}


\begin{table}[h!]
\small
\begin{center}
% \setlength\tabcolsep{3pt}
% \begin{tabular}{cccc}
% \thickhline Dataset & Step & Entities/Actions & Relations  \\ \hline
\begin{tabular}{ccc}
\thickhline Dataset & Entities/Actions & Relations  \\ \hline
\textsc{PubMedM\&M} & 70.54 & 51.94 \\
% \multirow{2}{*}{\textsc{PubMedM\&M}} & step-1 & 70.54 & 51.94 \\ 
% & step-2 & 88.19 & 77.67 \\ \hline

\textsc{ChemSyn} & 79.87 & 87.20 \\ 
% \multirow{2}{*}{\textsc{ChemSyn}} & step-1 & 79.87 & 87.20 \\ 
% & step-2 & 99.28 & 98.18 \\ 

\thickhline
\end{tabular}
\end{center}
\caption{\label{tab:iaa_results} Inter-Annotator Agreement ($F_1$ scores on Entity/Action Identification and Relation Extraction) of two annotation steps.}
\end{table}

\section{Hyper-parameter for Downstream Tasks}
\label{sec:hyper_para}
